# Supplementary material for: The Fiscal Cost of Public Debt and Government Spending Shocks
Source: arXiv:2309.07371 source file (2023-09-14)
Supplement: Supplementary file 1 [file appendix_subsample.tex]

\begin{tabular}{@{\extracolsep{10pt}}lccccc}
\toprule
\bottomrule
\\[-1.4ex]
 & $h = 0$ & $h = 4$ & $h = 8$ & $h=12$ & $h=16$ \\
\midrule
& \multicolumn{5}{c}{Pre WWII} \\ \cline{2-6} \\[-1.8ex]
IRF Spending: & & & & \\
\quad Baseline States & 0.98$^{***}$ & 1.25$^{***}$ & 1.18$^{***}$ & -0.12 & -1.49 \\
\quad Diff. Costly Debt & 0.46$^{***}$ & 0.04 & -1.16$^{***}$ & -0.38 & 0.70 \\
IRF Output:  & & & & \\
\quad Baseline States & 1.01$^{***}$ & 0.34 & -0.57 & -1.33$^{**}$ & -3.00$^{**}$ \\
\quad Diff. Costly Debt & -0.33 & 0.86 & 0.83 & 1.21 & 2.81 \\
Multipliers : & & & & \\
\quad Baseline States & 1.00$^{***}$ & 0.65$^{***}$ & 0.12 & 0.32 & 0.34 \\
\quad Diff. Costly Debt & -0.31 & -0.07 & 1.31$^{**}$ & 1.89 & 3.52 \\
\\[-1.4ex]
& \multicolumn{5}{c}{Post WWII} \\ \cline{2-6} \\[-1.8ex]
IRF Spending: & & & & \\
\quad Baseline States & 1.25$^{***}$ & 2.44$^{***}$ & 2.55$^{***}$ & 2.22$^{***}$ & -0.12 \\
\quad Diff. Costly Debt & 0.32$^{**}$ & -0.43 & -2.07$^{***}$ & -2.39$^{***}$ & 0.01 \\
IRF Output:  & & & & \\
\quad Baseline States & 1.12$^{***}$ & 1.89$^{***}$ & 1.87$^{***}$ & 1.83$^{***}$ & 0.75$^{**}$ \\
\quad Diff. Costly Debt & 0.14 & -0.47 & -1.55$^{***}$ & -1.88$^{***}$ & -0.37 \\
Multipliers : & & & & \\
\quad Baseline States & 0.96$^{***}$ & 0.85$^{***}$ & 0.78$^{***}$ & 0.81$^{***}$ & 0.85$^{***}$ \\
\quad Diff. Costly Debt & 0.08 & -0.17 & -0.04 & -0.08 & -0.04 \\
\\[-1.4ex]
& \multicolumn{5}{c}{Excluding GFC} \\ \cline{2-6} \\[-1.8ex]
IRF Spending: & & & & \\
\quad Baseline States & 1.07$^{***}$ & 2.21$^{***}$ & 2.77$^{***}$ & 2.43$^{***}$ & 0.21 \\
\quad Diff. Costly Debt & 0.51$^{***}$ & -0.71$^{***}$ & -2.59$^{***}$ & -2.76$^{***}$ & -0.30 \\
IRF Output:  & & & & \\
\quad Baseline States & 1.15$^{***}$ & 2.26$^{***}$ & 2.57$^{***}$ & 2.31$^{***}$ & 0.90$^{*}$ \\
\quad Diff. Costly Debt & -0.29 & -1.43$^{***}$ & -2.33$^{***}$ & -2.30$^{***}$ & -0.80 \\
Multipliers : & & & & \\
\quad Baseline States & 1.04$^{***}$ & 0.98$^{***}$ & 0.88$^{***}$ & 0.89$^{***}$ & 0.91$^{***}$ \\
\quad Diff. Costly Debt & -0.39 & -0.45$^{***}$ & -0.24 & -0.22 & -0.23 \\
\bottomrule
\end{tabular}
